# Supplementary material for: Figure Captioning with Reasoning and Sequence-Level Training
Source: arXiv:1906.02850 source file (2019-06-07)
Supplement: Supplementary file 1 [file supplement.tex]

\pdfoutput=1
\documentclass[11pt,a4paper]{article}
\usepackage[hyperref]{naaclhlt2019}
\usepackage{times}
\usepackage{latexsym}

\usepackage{url}

\aclfinalcopy % Uncomment this line for the final submission
%\def\aclpaperid{***} %  Enter the acl Paper ID here

%\setlength\titlebox{5cm}
% You can expand the titlebox if you need extra space
% to show all the authors. Please do not make the titlebox
% smaller than 5cm (the original size); we will check this
% in the camera-ready version and ask you to change it back.

\usepackage{comment}
\usepackage{soul}

\usepackage{helvet}  %Required
\usepackage{courier}  %Required
\usepackage{url}  %Required
\usepackage{graphicx}  %Required
\frenchspacing  %Required
\setlength{\pdfpagewidth}{8.5in}  %Required
\setlength{\pdfpageheight}{11in}  %Required
%PDF Info Is Required:
%\pdfinfo{
%	/Title (Figure Captioning with Reasoning and Sequence-Level Training)
%	/Authors}
%\setcounter{secnumdepth}{0} 

\usepackage{booktabs}
\usepackage{tabularx}
\usepackage{comment}

\usepackage{microtype}
\usepackage{graphicx}
\usepackage{subfigure}
\usepackage{booktabs} % for professional tables
\usepackage{wrapfig}

\usepackage{hyperref}

\usepackage[utf8]{inputenc} % allow utf-8 input
\usepackage[T1]{fontenc}    % use 8-bit T1 fonts
\usepackage{url}            % simple URL typesetting
\usepackage{amsfonts}       % blackboard math symbols
\usepackage{nicefrac}       % compact symbols for 1/2, etc.
\usepackage{subfigure}
\graphicspath{{figures/}}
\usepackage{xcolor}
\usepackage{adjustbox}
\usepackage{bm}
\usepackage{amsmath}
\usepackage{amssymb}
\usepackage{algorithm}
\usepackage{algorithmic}
\usepackage{multirow}
\usepackage{adjustbox}

\usepackage{bm}

\newcommand{\RN}[1]{%
	\textup{\lowercase\expandafter{\it \romannumeral#1}}%
}

\input{myMacros.tex}

\begin{document}

\appendix

\section{Appendix}
\label{sec:appendix}

\textbf{Templates}

Note that Table 1 in our paper only lists selected templates. In order to control the variation for either high-level description or relation description, we design templates output diverse captions based on known attributes about the figure.
For high-level caption (FigCAP-H), the total number of templates (i.e. the possible variation with the same meaning) is 228.

For relation caption (FigCAP-D), captions include relations among the labels in the figures. There are 5 different types of relations in vertical bar charts, horizontal bar charts and pie including: maximum, minimum, greater than, less than and median. For line plots and dotted line plots, there are 9 different types of relations (e.g, minimum area under the curve , smoothest, lowest value, etc) 

The number of templates (i.e. number of possible variation of the same meaning for relation description): summation of permutation of 5 and permutation of 9.

\end{document}
